# Supplementary material for: Proposed Method for Distinguishing Majorana Peak from Other Peaks: Tunneling Spectroscopy with Ohmic Dissipation using Resistive Electrodes
Source: arXiv:1310.4883 source file (2013-10-18)
Supplement: Supplementary file 1 [file supp_DissipativeMF_V1.pdf]

# Supplementary Information for "Tunneling Spectroscopy with Ohmic Dissipation : A Majorana Signature Filter"

Dong E. Liu
*Department of Physics and Astronomy, Michigan State University, East Lansing, Michigan 48824, USA*
(Dated: July 27, 2013)

In this supplementary information we will provide the details of the derivation of 1) the weak coupling RG equation for tunneling into a zero-energy impurity bound state (ZEIBS), 2) the relation to a Luttinger liquid model and low $T$ conductance for tunneling into a Majorana fermion zero mode, and 3) the phase correlation function $J(t)$ and $P(\omega)$ of Eq.(12) and (13) in the main text.

## I. DERIVATION OF THE WEAK COUPLING RG EQUATIONS FOR TUNNELING INTO ZEIBS

In this section, we will derive the weak coupling RG equations shown in Eq. (11) of the main text. The effective Hamiltonian describing the tunneling into a ZEIBS (i.e. Eq. (10) of the main text) is

$$\begin{aligned} H &= \sum_\sigma \frac{v_F}{4\pi}\int_{-\infty}^{\infty} dx\big(\partial_x\widetilde{\Phi}_\sigma(x)\big)^2 + \Big[y_{\mathrm{d},\sigma}\frac{F_\sigma}{\sqrt{2\pi}}e^{-i\widetilde{\Phi}_\sigma(0)/\sqrt{g}}\,d + y_{\mathrm{c},\sigma}\frac{F_\sigma}{\sqrt{2\pi}}e^{-i\widetilde{\Phi}_\sigma(0)/\sqrt{g}}d^\dagger + h.c.\Big] \\ &\quad + \frac{K_\sigma}{\sqrt{g}\pi}(d^\dagger d - 1/2)\partial_x\widetilde{\Phi}_\sigma(0). \end{aligned} \tag{S1}$$

To obtain the full scaling dimension of the tunneling $y_{\mathrm{d},\sigma}$ and $y_{\mathrm{c},\sigma}$, we first apply a unitary transformation [1]:

$$U = \exp\Big[i\frac{\widetilde{K}_\uparrow}{\sqrt{g}}(d^\dagger d - \frac{1}{2})\,\widetilde{\Phi}_\uparrow(x=0)\Big] \times \exp\Big[i\frac{\widetilde{K}_\downarrow}{\sqrt{g}}(d^\dagger d - \frac{1}{2})\,\widetilde{\Phi}_\downarrow(x=0)\Big], \tag{S2}$$

and then, the effective Hamiltonian becomes

$$\begin{aligned} H' = U^\dagger H U &= \sum_\sigma \Bigg(\frac{v_F}{4\pi}\int_{-\infty}^{\infty} dx\big(\partial_x\widetilde{\Phi}_\sigma(x)\big)^2 + \Big[y_{\mathrm{d},\sigma}\frac{F_\sigma}{\sqrt{2\pi}}e^{-i\frac{(1-\widetilde{K}_\sigma)}{\sqrt{g}}\widetilde{\Phi}_\sigma(0)}e^{i\frac{\widetilde{K}_{-\sigma}}{\sqrt{g}}\widetilde{\Phi}_{-\sigma}(0)}\,d + h.c.\Big] \\ &\quad + \Big[y_{\mathrm{c},\sigma}\frac{F_\sigma}{\sqrt{2\pi}}e^{-i\frac{(1+\widetilde{K}_\sigma)}{\sqrt{g}}\widetilde{\Phi}_\sigma(0)}e^{-i\frac{\widetilde{K}_{-\sigma}}{\sqrt{g}}\widetilde{\Phi}_{-\sigma}(0)}\,d^\dagger + h.c.\Big] \\ &\quad + \Big(\frac{K_\sigma}{\sqrt{g}\pi} - \frac{v_F\widetilde{K}_\sigma}{2\sqrt{g}}\Big)(d^\dagger d - 1/2)\partial_x\widetilde{\Phi}_\sigma(0)\Bigg) \end{aligned} \tag{S3}$$

If we choose the dimensionless parameter $\widetilde{K}_\sigma = 2K_\sigma/(\pi v_F)$, the density interaction in $H'$ vanishes ( but it can be generated from the scaling processes). Because of the relation:

$$\langle \exp(iA\widetilde{\Phi}_\sigma(0,t))\exp(-iA\widetilde{\Phi}_\sigma(0,0))\rangle \sim \frac{1}{t^{A^2}} \tag{S4}$$

and the impurity $d$ does not contribute to the scaling dimension ([...]), the full scaling dimension of the tunneling operator is

$$\begin{aligned} [\hat{O}_{d,\sigma}] &= \Big[\tfrac{F_\sigma}{\sqrt{2\pi}}e^{-i\frac{(1-\widetilde{K}_\sigma)}{\sqrt{g}}\widetilde{\Phi}_\sigma(0)}e^{i\frac{\widetilde{K}_{-\sigma}}{\sqrt{g}}\widetilde{\Phi}_{-\sigma}(0)}\,d + h.c.\Big] = \tfrac{(1-\widetilde{K}_\sigma)^2}{2g} + \tfrac{(\widetilde{K}_{-\sigma})^2}{2g} \\ [\hat{O}_{c,\sigma}] &= \Big[\tfrac{F_\sigma}{\sqrt{2\pi}}e^{-i\frac{(1+\widetilde{K}_\sigma)}{\sqrt{g}}\widetilde{\Phi}_\sigma(0)}e^{-i\frac{\widetilde{K}_{-\sigma}}{\sqrt{g}}\widetilde{\Phi}_{-\sigma}(0)}\,d^\dagger + h.c.\Big] = \tfrac{(1+\widetilde{K}_\sigma)^2}{2g} + \tfrac{(\widetilde{K}_{-\sigma})^2}{2g} \end{aligned} \tag{S5}$$

We then obtain the weak coupling RG equations for $y_{d,\sigma}$ and $y_{c,\sigma}$, i.e. the first two equations of Eq. (11) in the main text:

$$\begin{aligned} \frac{dy_{d,\sigma}}{d\ln l} &= \Big(1 - \frac{(1-\widetilde{K}_\sigma)^2}{2g} - \frac{(\widetilde{K}_{-\sigma})^2}{2g}\Big)y_{d,\sigma}, \\ \frac{dy_{c,\sigma}}{d\ln l} &= \Big(1 - \frac{(1+\widetilde{K}_\sigma)^2}{2g} - \frac{(\widetilde{K}_{-\sigma})^2}{2g}\Big)y_{c,\sigma}, \end{aligned} \tag{S6}$$

where $l$ is a short-time cutoff in the scaling. The scaling dimension of the density interaction operator $[\hat{O}_{K\sigma}] = [(d^\dagger d - 1/2)\partial_x \widetilde{\Phi}_\sigma(0)] = 1$ [2, 3], they are marginal operators with vanishing leading order terms in RG equations. Therefore, we have to consider the second order terms in the RG equations. Operator product expansion (OPE) [2, 4] provides a powerful way to derive the second order terms in the RG equations (also see [5] for review). Consider an action $S_0$ describing a non-interacting theory (or a conformal field theory), and a set of boundary perturbations with dimensionless coupling constants $g_i$:

$$S = S_0 + \sum_i g_i \int dr \hat{O}_i(r). \tag{S7}$$

For our impurity problem, the the weak coupling RG equations up to the second order is [2, 4] :

$$\frac{dg_k}{d\ln l} = (1 - [\hat{O}_i])g_k - \sum_{i,j} C_{i,j,k} g_i g_j \tag{S8}$$

where $C_{i,j,k}$ are the operator product expansion coefficients [2, 4, 5] (which are pure numbers):

$$\hat{O}_i(r)\hat{O}_j(r') = \sum_k \frac{C_{i,j,k}\hat{O}_k(r)}{(r-r')^{[\hat{O}_i]+[\hat{O}_j]-[\hat{O}_k]}}, \tag{S9}$$

We now will calculate these coefficients for our density interaction operator $\hat{O}_{K\sigma}$, which can be generated by the product of $\hat{O}_{d,\sigma}$ operators and $\hat{O}_{c,\sigma}$ operators. We first define a set of dimensionless parameters: $\widetilde{y}_{d,\sigma} = y_{d,\sigma} l/\sqrt{2\pi}$, $\widetilde{y}_{c,\sigma} = y_{c,\sigma} l/\sqrt{2\pi}$, and $\widetilde{K}_\sigma = 2K_\sigma/(\pi v_F)$. By using the OPE relation $e^{iA\widetilde{\Phi}_\sigma(x)} e^{-iA\widetilde{\Phi}_\sigma(x')} \sim -A\partial_x \widetilde{\Phi}_\sigma(x)/(x-x')^{A^2-1}$, we can obtain the leading order terms in OPE:

$$\begin{aligned}
\hat{O}_{d,\sigma}(x)\hat{O}_{d,\sigma}(x') &\sim -2(d^\dagger d - \frac{1}{2})\left[\frac{\frac{1-\widetilde{K}_\sigma}{\sqrt{g}}\partial_x\widetilde{\Phi}_\sigma(x)}{(x-x')^{2[\hat{O}_{d,\sigma}]-1}} - \frac{\frac{\widetilde{K}_{-\sigma}}{\sqrt{g}}\partial_x\widetilde{\Phi}_{-\sigma}(x)}{(x-x')^{2[\hat{O}_{d,\sigma}]-1}}\right] \\
\hat{O}_{c,\sigma}(x)\hat{O}_{c,\sigma}(x') &\sim -2(d^\dagger d - \frac{1}{2})\left[-\frac{\frac{1+\widetilde{K}_\sigma}{\sqrt{g}}\partial_x\widetilde{\Phi}_\sigma(x)}{(x-x')^{2[\hat{O}_{c,\sigma}]-1}} - \frac{\frac{\widetilde{K}_{-\sigma}}{\sqrt{g}}\partial_x\widetilde{\Phi}_{-\sigma}(x)}{(x-x')^{2[\hat{O}_{c,\sigma}]-1}}\right]
\end{aligned} \tag{S10}$$

We then obtain the weak coupling RG equations for $\widetilde{K}_\sigma$, i.e. the last equation of Eq. (11) in the main text

$$\frac{d\widetilde{K}_\sigma}{d\ln l} = 2(1-\widetilde{K}_\sigma)\widetilde{y}_{d,\sigma}^2 - 2(1+\widetilde{K}_\sigma)\widetilde{y}_{c,\sigma}^2 - 2\widetilde{K}_\sigma\widetilde{y}_{d,-\sigma}^2 - 2\widetilde{K}_\sigma\widetilde{y}_{c,-\sigma}^2. \tag{S11}$$

Note that since $\widetilde{K}_\sigma$ are dimensionless, we have to use the dimensionless parameters $\widetilde{y}_{d,\sigma}$ and $\widetilde{y}_{c,\sigma}$ here.

## II. THE RELATION TO LUTTINGER LIQUID MODEL AND THE LOW $T$ CONDUCTANCE FOR TUNNELING INTO A MF

Similarly to the procedure for ZEIBS (i.e. the derivation of Eq. (9) of the main text), one can rewrite the Hamiltonian for the tunneling into a Majorana fermion (i.e. Eq. (5) of the main text) in a bosonized form

$$H = \frac{v_F}{4\pi}\int_{-\infty}^{\infty} dx \big(\partial_x \Phi(x)\big)^2 + \Big[y_{\mathrm{k}} \frac{Fe^{-i\Phi(0)}}{\sqrt{2\pi}}\gamma_1 e^{-i\phi} + h.c.\Big] \tag{S12}$$

Note that even for a spinful lead, MF couples to only a single channel, which is the linear combination of the spin up and down channels. We apply the exactly the same process for ZEIBS in the main text: we can combine the two bosonic fields and introduce a new field [6–8]: $\widetilde{\Phi}_\sigma(x) = \sqrt{g}(\Phi_\sigma(x) + \phi(x))$ with $g = 1/(1+2r)$, which satisfies $\langle e^{-i\widetilde{\Phi}_\sigma(x=0,t)} e^{i\widetilde{\Phi}_\sigma(x=0,0)}\rangle \sim t^{-1}$. Then, the Hamiltonian becomes

$$H = \frac{v_F}{4\pi}\int_{-\infty}^{\infty} dx \big(\partial_x \widetilde{\Phi}(x)\big)^2 + \Big[y_{\mathrm{k}} \frac{F}{\sqrt{2\pi}} e^{-i\widetilde{\Phi}(0)/\sqrt{g}}\gamma_1 + h.c.\Big], \tag{S13}$$

The original model is thus mapped to a natural physical system: a MF zero mode coupled to a spinless Luttinger liquid with interaction parameter $g = 1/(1+2r)$ [2, 3]. As shown in Ref. [9],the zero voltage bias conductance for this MF-spinless Luttinger liquid model scales as $2e^2/h - G \sim T^{2(2g-1)} = T^{(2-4r)/(1+2r)}$ near the strong coupling fixed point (i.e. low $T$ limit).

## III. THE PHASE CORRELATION FUNCTION $J(t)$ AND $P(\omega)$ OF EQ.(12) AND (13) IN THE MAIN TEXT

The phase correlation of the tunneling junction with total environmental impedance $Z_t(\omega)$, can be written as (please refer to section 3.3 of Ref. [10] for review)

$$J(t) = \langle\phi(t)\phi(0)\rangle - \langle\phi^2\rangle = 2\int_0^\infty \frac{d\omega}{\omega}\frac{\mathrm{ReZ_t}(\omega)}{R_K}\Big\{\coth\Big(\frac{\omega}{2T}\Big)[\cos(\omega t)-1] - i\sin(\omega t)\Big\}. \quad \text{(S14)}$$

Here, the total impedance $Z_t(\omega) = 1/(iC + Z(\omega)^{-1})$, where $C$ is the junction capacitance in parallel with the external impedance $Z(\omega)$. For ohmic dissipation, we have $Z(\omega) = R$, then the correlation becomes

$$J(t) = 2r\int_0^\infty \frac{d\omega}{\omega}\frac{1}{1+(\frac{\omega}{\omega_R})^2}\Big\{\coth\Big(\frac{\omega}{2T}\Big)[\cos(\omega t)-1] - i\sin(\omega t)\Big\}, \quad \text{(S15)}$$

where $\omega_R = 1/(RC)$ is an cutoff of the effective circuit (we choose $\omega_R = 1.0$ in numerics of Fig. 3 of the main text). For very large cutoff, the real part of the total impedance can be treated as a constant, which however results in an ultraviolet divergence in the integral. To obtain an analytic result of this integral, we restore this natural cutoff with an ultraviolet regularization $e^{-\omega/\omega_R}$. Here, we replace the original lorentzian with an exponential function, which is valid for very large cutoff (i.e. $\omega_R/T \gg 1$). Then, we reach the simple analytic result for finite $T$:

$$J(t) = 2r\ln\Big[\frac{\pi T/i\omega_R}{\sinh[\pi T(t - i/\omega_R)]}\Big], \quad \text{(S16)}$$

The correlation function $J(t)$ for $T = 0$ and $t \to \infty$ can be obtained by using a more rigorous method [10], which include an extra constant compared to Eq. (S16) in the limit $T = 0$ and $t \to \infty$. For our purpose, this constant difference only induces a constant pre-factor and do not affect the main physics at least for $\omega_R/T \gg 1$. We then calculate its Fourier transformation $P(\omega)$:

$$\begin{aligned} P(\omega) &= \frac{1}{2\pi}\int_{-\infty}^{\infty} dt \exp[i\omega t + J(t)] \\ &= \frac{1}{2\pi}\Big(\frac{\pi T}{i\omega_R}\Big)^{2r}\int_{-\infty}^{\infty} dt e^{i\omega t}\frac{1}{\big(\sinh[\pi T(t - i/\omega_R)]\big)^{2r}} \\ &= \frac{2^{2r-1}}{2\pi\omega_R\Gamma(2r)}\Big(\frac{\pi T}{\omega_R}\Big)^{2r-1} e^{\frac{\omega}{2T}}\big|\Gamma(r + i\frac{\omega}{2\pi T})\big|^2 \end{aligned} \quad \text{(S17)}$$

where we take $1/\omega_R \to 0$ in the integral from the second line to the third line.

---


[1] V. J. Emery and S. Kivelson, Phys. Rev. B **46**, 10812 (1992).
[2] D. Senechal, in *Theoretical Methods for Strongly Correlated Electrons* (2003), arXiv:cond-mat/9908262.
[3] T. Giamarchi, *Quantum Physics in One Dimension* (Oxford Univ. Press, 2004).
[4] J. Cardy, *Scaling and Renormalization in Statistical Physics* (Cambridge Univ. Press, 1996), page 83-90.
[5] M. E. Peskin and D. V. Schroeder, *An Introduction to Quantum Field Theory* (Westview Press, 1995), p. 612-615.
[6] S. Florens, P. Simon, S. Andergassen, and D. Feinberg, Phys. Rev. B **75**, 155321 (2007).
[7] K. Le Hur and M.-R. Li, Phys. Rev. B **72**, 073305 (2005).
[8] H. T. Mebrahtu, I. V. Borzenets, D. E. Liu, H. Zheng, Y. V. Bomze, A. I. Smirnov, H. Baranger, and G. Finkelstein, Nature **488**, 61 (2012).
[9] L. Fidkowski, J. Alicea, N. H. Lindner, R. M. Lutchyn, and M. P. A. Fisher, Phys. Rev. B **85**, 245121 (2012).
[10] G.-L. Ingold and N. Yu.V., in *Single Charge Tunneling: Coulomb Blockade Phenomena in Nanostructures*, edited by H. Grabert and M. H. Devoret (Plenum Press, New York, 1992), vol. 294, pp. 21–107, arXiv:cond-mat/0508728.
